# Supplementary material for: Learning Deep Optimal Embeddings with Sinkhorn Divergences
Source: arXiv:2209.06469 source file (2022-09-14)
Supplement: Supplementary file 1 [file paper_supp.tex]

\section{sup}

hahah
